# Supplementary material for: The Collective Burst Mechanism of Angular Jumps in Liquid Water
Source: arXiv:2206.04298 ancillary file (2022-07-11)
Supplement: Supplementary file 1 [file SupplementaryInformation.pdf]

# Supplementary Information for

## The Collective Burst Mechanism of Angular Jumps in Liquid Water

**Adu Offei-Danso, Uriel N. Morzan, Alex Rodriguez, Ali Hassanali, Asja Jelic**

**E-mail: asja@ictp.it**

### Supporting Information Text

### Methods

**Correlation in time between concurrent large angular swings.** In Fig.S3, we looked at the water molecules that concurrently perform large-amplitude swings and examined how much correlated are the parts of their angular trajectories around the times of these large swings. In particular, we calculated the Pearson coefficients between the HH and DP vector time series of different molecules over a certain time interval of length $dT$ that encompasses the detected large angular swings. In order to do that, for every molecule, we selected the time series of the component of the HH or DP vector with the largest change in magnitude during that time interval $dT$. In that way, we approximated the angular motion of each water molecule by looking at the direction with the most significant change within the time interval of consideration. We found that an average duration of a large-amplitude angular swing is around 0.1 ps (see Fig. 4A and Fig.S6A), therefore, we take $dT$ to be 0.1 ps or longer.

For varying time interval widths $dT$, ranging from 0.1 ps to 100 ps, we extracted the Pearson correlation coefficients between molecules undergoing large angular swings greater than $60^{\circ}$, as described above. We then constructed probability density estimates from the Pearson correlation coefficients. On average, 50 out of 1019 waters are found to undergo large angular fluctuations within 0.1ps. Therefore, for these results to be statistically significant, we considered different time intervals of length $dT$ in the trajectory, by shifting the initial time of the window of consideration by $dT$, in order to avoid overlapping statistics. Each probability density estimate was constructed using 10,000 Pearson coefficients. Finally, the probability distributions for molecules undergoing large angular swings were then contrasted with distributions generated by computing the Pearson correlation coefficients between all water molecules over time interval $dT$ in a similar manner. The results of this analysis are shown in Fig.S3.

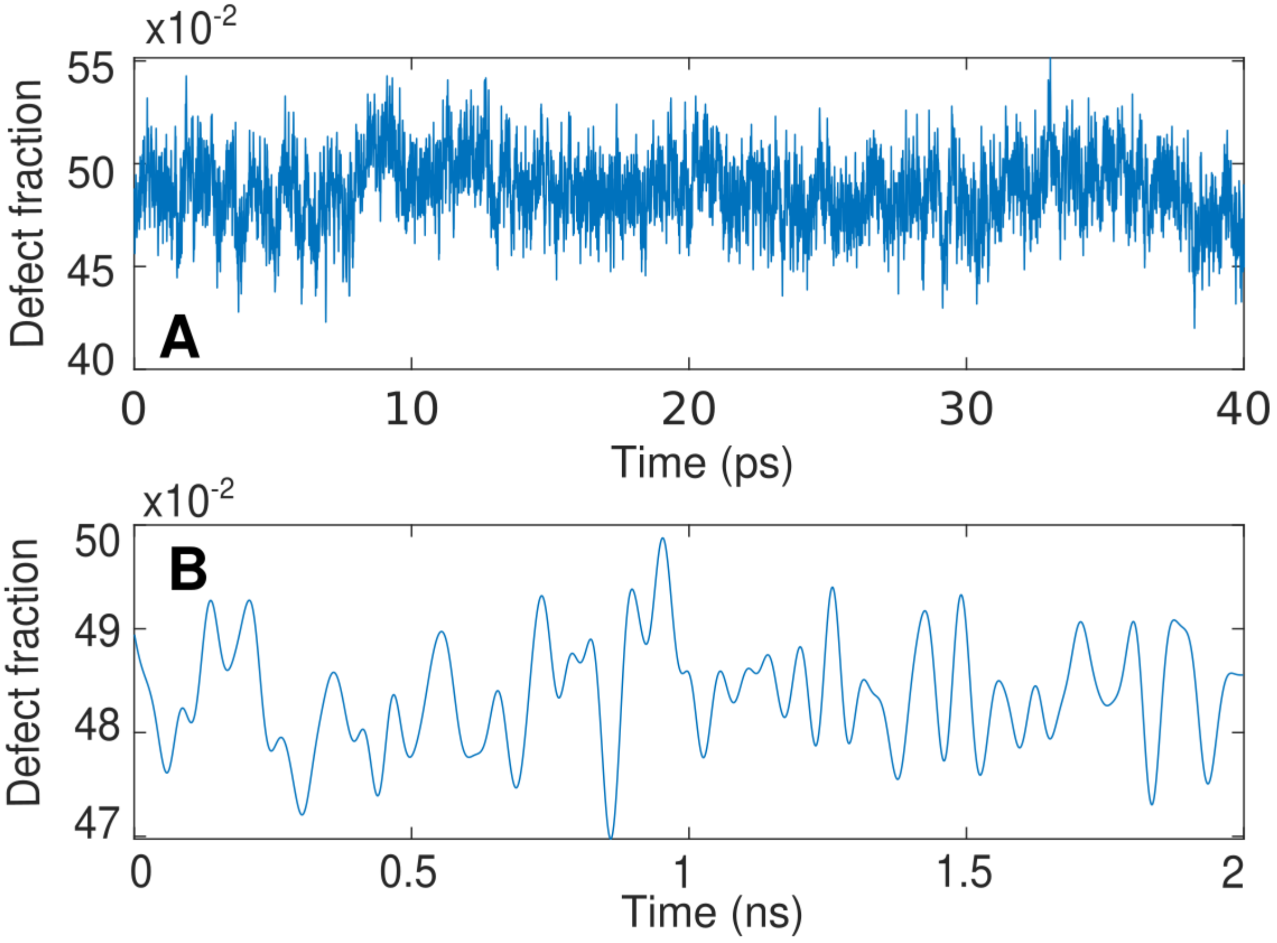


**Fig. S1.** Fluctuations in the local topology of the water hydrogen bond network. (A) Unfiltered times series of the fraction of defects (water molecules with non-tetrahedral local topology) on short time scales shows large defect oscillations, reflecting processes in the network that lead to the creation and annihilation of up to 10-20 defective water molecules in the network. (B) Time series of the fraction of defects over a total period of 2 ns of the MD simulation.

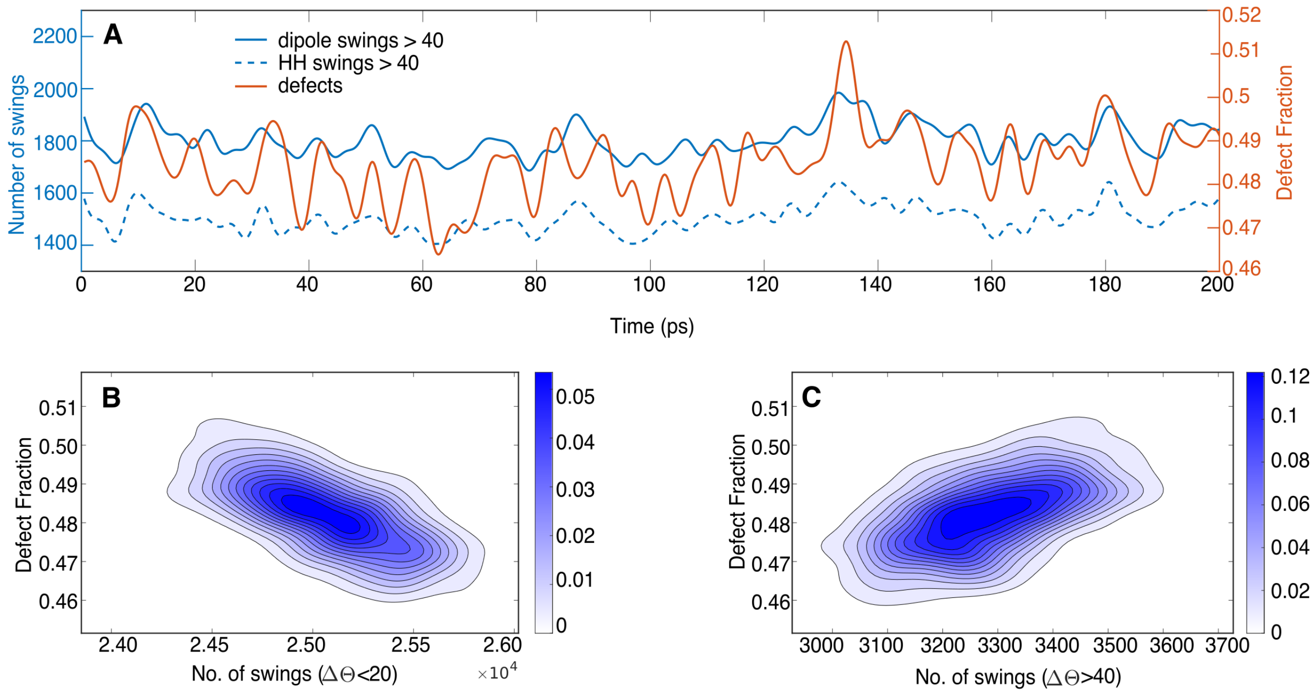


**Fig. S2.** Correlation between the number of simultaneous large angular swings and the fluctuations in the local topology of the water H-bond network. This is similar to Fig.3 in the main text, except that here we reduce the threshold for the minimal magnitude of what is considered a large swing from $60^\circ$ to $40^\circ$, therefore including more angular swings. (A) Time series of the number of molecules in the H-bond network performing large angular swings (amplitude larger than $40^\circ$) at each moment of time as detected from the observation of the dipole vector (blue full line) and HH vector (blue dashed line). At each moment of time, we count the number of swings happening in the system within a time window of 1ps around it. We superimpose these time series with the time series of the fraction of molecules in the H-bond network that are defective, i.e. with non-tetrahedral local topology (red). As in the case of swings with $\Delta\Theta > 60$, also here we observe fluctuations of the order of tens of picoseconds in all three curves that often appear to be correlated in time, even though the peaks of the number. (B) Density plot of the fraction of defects in the H-bond network with respect to the number of molecules in the network performing small angular swings ($\Delta\Theta < 20$) within 1ps. Anti-correlation between these two quantities means that when there are more molecules with defective local topology, the less small-amplitude angular swings occur in the H-bond network. We find the correlation coefficient to be $-0.7390 \pm 0.0089$, with $p < 0.01$. (C) Density plot of the fraction of defects in the H-bond network with respect to the number of large-amplitude angular swings ($\Delta\Theta > 40^\circ$) within 1 ps. Correlation between these two quantities indicates that the more the local topology in the H-bond network is defective, the larger is the number of molecules that perform large-amplitude angular swings. The correlation coefficient found is $0.57 \pm 0.02$, with $p < 0.01$

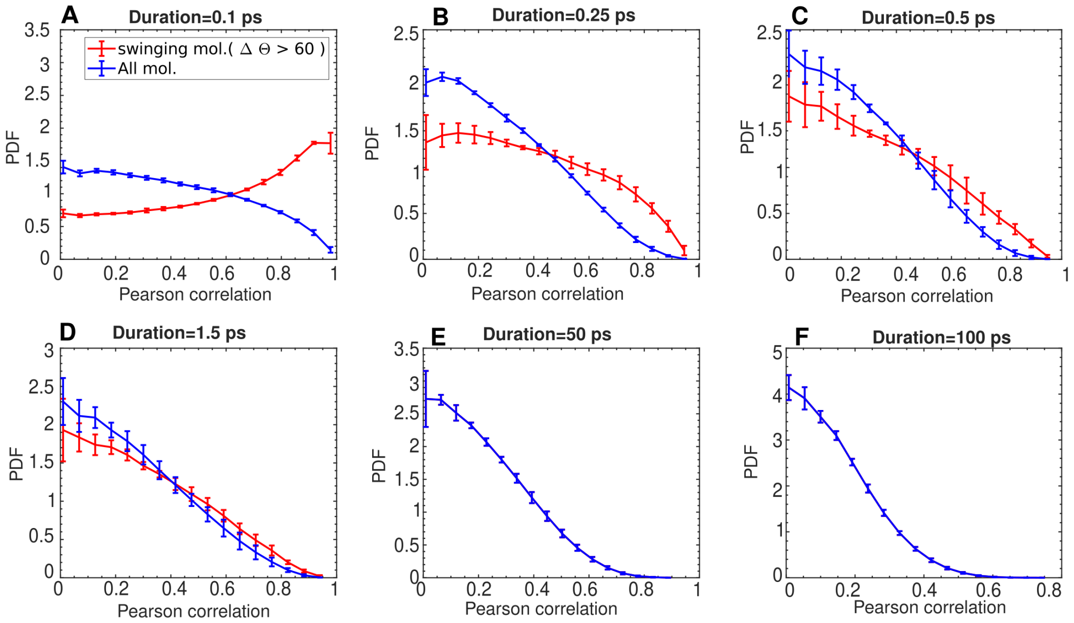


**Fig. S3.** Correlation in time of the angular trajectories of water molecules concurrently performing large swings ($\Delta\Theta > 60^{\circ}$). (A,B,C) In the top three panels, we plot the probability distribution functions of the Pearson correlation coefficient between the HH vector trajectories of length 0.10, 0.25, and 0.50 ps encompassing the angular swings. We show the difference in the correlations between the time series of the molecules with large-amplitude swings (red), with respect to those of all molecules that perform angular swings (blue) within the time window of interest. While for the shortest time interval the correlation between the large swings (red curves) is typically high (peak of the curve is close to 1), as the time interval increases, the time series become more and more uncorrelated and we find that the two distributions almost overlap for 0.5 ps. On the contrary, when we look at the same length trajectories for any other two molecules, they are typically much less correlated (blue curves) even for short times, as expected since motion of any two water molecules in the system is not expected to be correlated. (D,E,F) Bottom panels show the distributions of the Pearson correlation coefficient for the parts of the trajectories of length 1.5, 50, and 100 ps, respectively. While the distributions for large-amplitude swings overlap with the ones of all the molecules, the fat tale that we find for intermediate times becomes less and less pronounces and at the order of 100 ps the time series become less and less correlated.

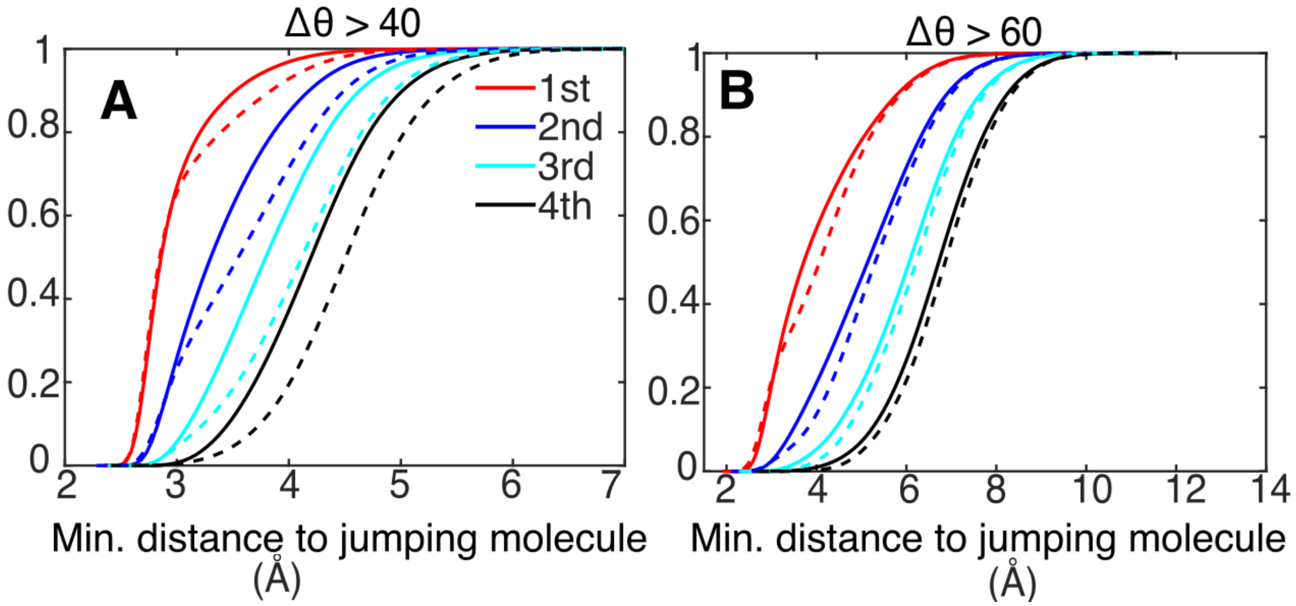


**Fig. S4.** Cumulative distribution functions (CDFs) of distances to the n-th nearest jumping waters, for jumps with amplitude $\Delta\Theta > 40^{\circ}$ and $\Delta\Theta > 60^{\circ}$, are shown by full lines in panels (A) and (B), respectively. These results are contrasted with CDFs of the n-th nearest neighbor distances between randomly selected molecules (dashed lines). We obtained the CDFs from the probability distribution functions shown in Fig.4C,D in the main text. While for large jumps with $\Delta\Theta > 60^{\circ}$ the difference between jumping and random molecules is visible, the difference becomes evident when we include also large jumps with $\Delta\Theta > 40^{\circ}$.

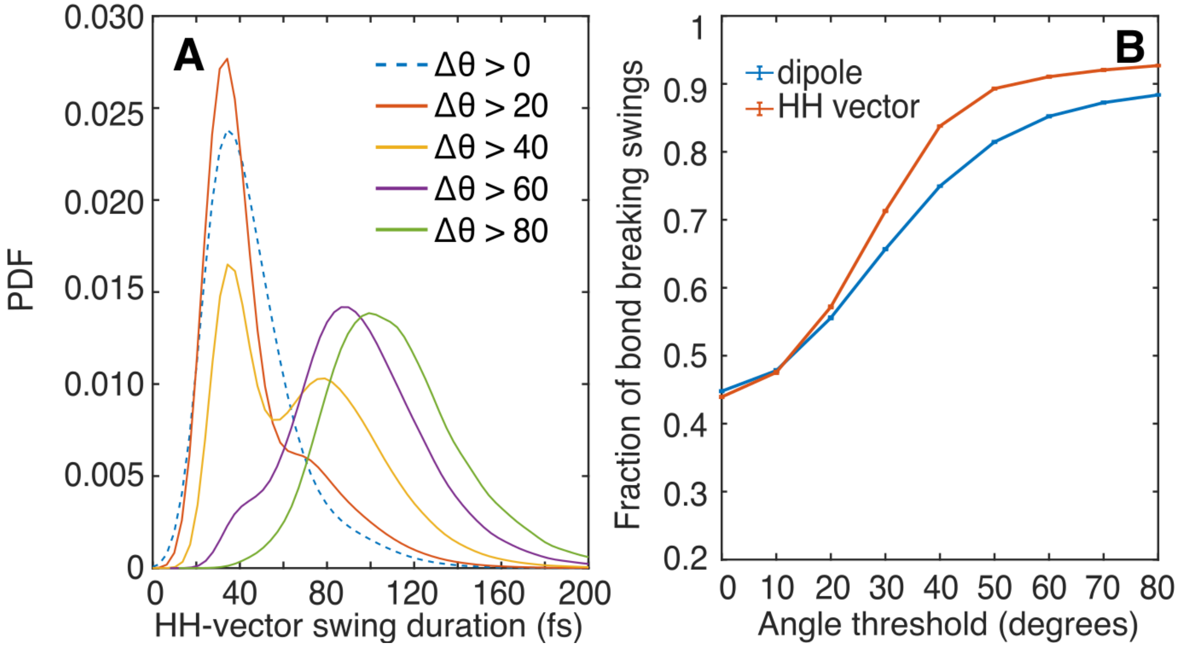


**Fig. S5.** Analysis of the angular swings duration, magnitude, and H-bond network local topology. (A) Probability distributions of duration $\Delta t$ of swings with the angular magnitude $\Delta\Theta$ greater than a certain threshold, detected from HH vectors time series, respectively. (B) Fraction of events in which we detect H-bond breaking, depending on the angular swing amplitude. The x-axis represents a threshold angle for the HH (red) and dipole (blue) vector, so that we count all swings with an amplitude larger than the threshold value. For swings with large amplitudes, most events involve hydrogen bond breaking.

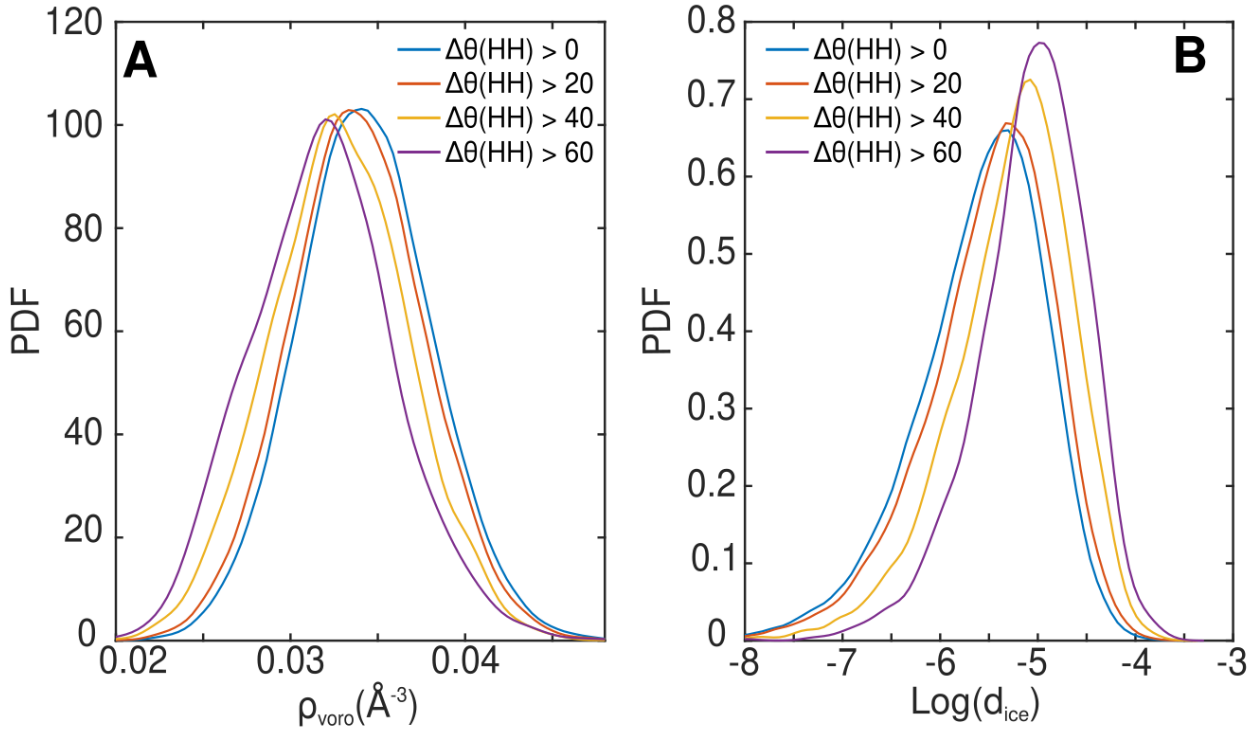


**Fig. S6.** (A) Probability distributions of the Voronoi density, $\rho_{\text{voro}}$, for the water molecules undergoing angular swings constrained by an HH-vector magnitude threshold. The probability distributions shifts towards lower local densities as we restrict ourselves to swings with the larger angular magnitude. (B) Probability distributions measuring the extent of the similarity of the local environments generated during angular jumps in liquid water, to that in hexagonal ice, namely $\log(d_{\text{ice}})$. Local environment of large angular swings with magnitude threshold $\Delta\theta > 60^{\circ}$ tends to be more disordered (less negative $\log(d_{\text{ice}})$) with respect to that of the small angular swings.

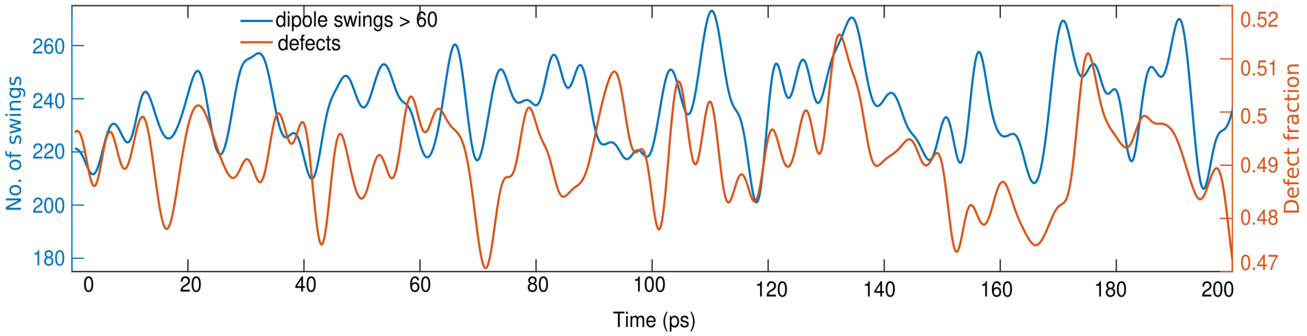


**Fig. S7.** Correlation between the number of simultaneous large angular swings and the fluctuations in the local topology of the water H-bond network of an MB-pol simulation of 512 water molecules at 298K(1). (A) Time series of the number of molecules in the H-bond network performing large angular swings (amplitude larger than $60^{\circ}$) at each moment of time as detected from the observation of the dipole vector (blue full line). At each moment of time, we count the number of swings happening in the system within a time window of 1ps around it. We superimpose this time series with that of the fraction of molecules in the H-bond network that are defective, i.e. with non-tetrahedral local topology (red). As in the case of swings with $\Delta\Theta > 60^{\circ}$, also here we observe fluctuations of the order of tens of picoseconds in all three curves that often appear to be correlated in time.

 

## References

1. V Babin, C Leforestier, F Paesani, Development of a "first principles" water potential with flexible monomers: Dimer potential energy surface, vrt spectrum, and second virial coefficient. *J. chemical theory computation* **9**, 5395–5403 (2013).
